# Supplementary material for: Augmented World Models Facilitate Zero-Shot Dynamics Generalization From a Single Offline Environment
Source: arXiv:2104.05632 source file (2021-08-03)
Supplement: Supplementary file 1 [file appendix_theory.tex]

\section{Theoretical Results}

If we decide to.
